# Supplementary material for: Topological Crystalline Bose Insulator in Two Dimensions via Entanglement Spectrum
Source: arXiv:1507.00348 source file (2015-07-10)
Supplement: Supplementary file 1 [file AppendixB_backup.tex]

\section{Symmetry action on free-boson CFT}
\label{Appendix:CFT}
The action of the symmetry on the edge degrees of freedom was used in Section
\ref{sec:symmetry} to construct topological invariants that
explain the double degeneracy of the entanglement spectrum for odd $W$ cylinders.
The gapless CFT structure of the edge cannot be explained using these invariants.
To argue that the gapless edge persists away from fine-tuned points, we need to use additional
information about how the symmetry interacts with the one-dimensional structure of the edge.
For on-site symmetries, Ref.~\onlinecite{LevinGu} proposed that the edges of 2D SPTs have anomalous symmetry
implementations that can be used to explain their gaplessness,
a proposal that has been elaborated on by several authors \cite{chen2014, else2014, williamson2014}. These proposals do not extend straightforwardly to lattice symmetry protected phases.
%But some attempts to extend it are \cite{hsieh2014, cho2015} which are not straightforward...

One source of additional information about the symmetry action on the edge is the identification of the
CFT primaries and descendants in the entanglement spectrum as shown in Figures~\ref{fig:EEIdentify} and \ref{fig:EEIdentifyPi}. While the relative entanglement energies and momenta that appear in the spectrum are fixed by the CFT structure and are independent of the microscopic implementation of the edge, the fact that some primaries appear shifted by momentum $\pi$ is not - it tells us that the corresponding primary states are odd under translation by one edge unit cell. We can confirm this by computing the edge symmetry action $V_T$ of translation in the canonical basis. Similarly, using the numerical form of the symmetry actions $V_g$ in the canonical basis,
we can determine the action of each symmetry on the CFT primary states
\begin{equation}
\ket{e, m} \sim \ e^{i(e \phi + m \theta)} \ket{0}.
\end{equation}
From this information, we can infer how the symmetries act on the free boson fields $\phi$ and $\theta$ that
appear in the low energy effective field theory description of the edge. (Under our conventions,
$\phi$ and $\theta$ are periodic with period $2\pi$, while $e$ and $m$ take integer values.)
For example, since $e$ is the \uone{} charge of the primary state $\ket{e, m}$, we can read off that the implementation of charge symmetry $V_{\varphi}$ in the free-boson theory is $\phi \to \phi + \varphi$,  $\theta \to \theta$.
Similarly, translation $T$ by one unit cell around the cylinder induces the following action on the edge variables:
\begin{gather}
\ket{e, m} \to e^{i K(e, m)} \ket{e, m} \sim (-1)^m \ket{e, m} \nonumber\\
 e^{i(e \phi + m \theta)} \to e^{i e\phi + m (\theta + \pi)} \nonumber \\
 \phi(x) \to \phi(x+1) \nonumber \\
 \theta(x) \to \theta(x+1) + \pi
\label{eq:cftsym2}
\end{gather}

We can also determine the action of the anti-unitary protecting symmetry $V_{\varPi \I_y}$ in this language.
Since the operation must flip both charge $e$ and momentum $K_y = em$ by virtue of being a pairing between left and right Schmidt states, with the relative phase fixed by $V_{\varPi \I_y} V_{\varPi \I_y}^* = -I$,
this is consistent with the following symmetry description for $V_{\varPi \I_y}$:
\begin{gather}
 \ket{e, m} \to (-1)^e\ket{-e, m} \nonumber \\
  e^{i(e \phi + m \theta)} \to e^{-i(-e \phi + e\pi + m \theta)} \nonumber \\
 \phi \to \phi + \pi \nonumber \\
 \theta \to -\theta
 \label{eq:cftsym1}
\end{gather}

Following Ref.~\onlinecite{LevinGu}, we can argue that the edge is protected by symmetries if each possible perturbation to the edge explicitly or spontaneously breaks the symmetry. The behavior of the edge theory under the possible pertubations is informed by previous analysis of bosonized one-dimensional systems \cite{giamarchi}.

Generic perturbations to the CFT edge are formed by operators $$H_{e, m} = U(x)\cos(e \phi + m \theta - \alpha(x)),$$ where $e, m$ are integers and $U(x)>0$ can be chosen by picking $\alpha(x)$ appropriately.
When the pertubation has a large coefficient, it has the effect of pinning the value of
$e \phi(x) + m \theta(x)$ to $\alpha(x) \mod 2 \pi$. This may be inconsistent with the symmetry implementation above, in case we say that the perturbation (explicitly or spontaneously) breaks the symmetry.

For example, by imposing $\varPi \I_y$, we find that pinning
\begin{equation*}
e \phi(x) + m \theta(x) \equiv \alpha(x)
\end{equation*}
also implies
\begin{equation*}
e \phi(x) + e\pi - m \theta(x) \equiv \alpha(x)
\end{equation*}
and hence
\begin{equation}
2m \theta(x) \equiv \pi e.
\end{equation}
If $m$ is not zero, then the value of $\theta(x)$ is pinned to one of the $2 m$ constant values
$$\theta(x) \equiv \pi e + \frac{2\pi}{2m} k.$$
$\theta(x)$ should not jump between these values, since the free boson action penalizes $(\nabla\theta)^2$. But pinning $\theta$ to a constant value is inconsistent with translation symmetry, since using translation symmetry $\theta(x) \equiv c \implies \theta(x+1)+\pi \equiv c$.
Thus perturbations with $m=0$ are forbidden by translation and $\varPi \I_y$.

If instead we add a perturbation with $m=0, e\neq0$, imposing $\varPi \I_y$, we find that $\phi(x)$ is pinned
\begin{equation*}
e \phi(x) \equiv \alpha(x).
\end{equation*}
Then $\phi(x)$ spontaneously chooses one of the $e$ values
$$\phi(x) \equiv \alpha(x) + \frac{2\pi}{e} k,$$
which is inconsistent with the symmetry $\varPi \I_y$, which shifts the value of $\phi$.

This argument suggests that the CFT structure of the edge is protected by $\varPi \I_y$ and translation, i.e. that any (possibly large) perturbation that gaps the edge explicitly or spontaneously breaks one of these symmetries.

We can also analyze whether the gapless edge mode is stable, by using the scaling dimensions of the perturbations to determine if {\em small} symmetry preserving perturbations lead to spontaneous symmetry breaking on the edge. Using the measured Luttinger parameter $\kappa \approx 1.6$, the scaling dimension
$\Delta = \frac{e^2}{4\kappa} + \kappa m^2$ is relevant for the primaries with $(e, m) = (1, 0), (2, 0), (3, 0), (0, 1), (1, 1)$. One can check that the perturbation
$$H_{2, 0} = U\cos(2 \phi - \alpha)$$
preserves translation symmetry and $\varPi \I_y$ and is relevant, so the edge is unstable to this perturbation.
Adding this perturbation at arbitrarily small levels should gap the edge, pin the field $\phi$, and spontaneously break charge parity symmetry.
